# Supplementary material for: SIMformer: Single-Layer Vanilla Transformer Can Learn Free-Space Trajectory Similarity
Source: arXiv:2410.14629 source file (2024-10-18)
Supplement: Supplementary file 1 [file appendix.tex]

\setcounter{table}{0} % 将表格计数器重置为0
\setcounter{section}{1}
\setcounter{figure}{0}
\pagenumbering{gobble}

\section*{Appendix}

\subsection{Approximation Error} \label{sec:appro_err}
Considering all prior works have only evaluated on downstream top-k similarity search task. However, trajectory similarity learning is essentially a regression task---evaluating the accuracy of the regression is crucial. Therefore, we assessed the MSE between the predicted similarity and the ground truth similarity for each model, presenting the results in \autoref{tab:appro_err}. It is evident that SIMformer significantly outperforms the baselines. 
The reason for this superior performance is that SIMformer is trained solely using the MSE loss without distinguishing between positive and negative samples. In contrast, the baseline models employ triplet loss, which prioritizes positive instances and introduces a margin threshold for negative instances. Consequently, when negative instances diverge adequately from the anchor trajectory, the optimization process halts. While this approach can enhance downstream top-$k$ similarity search tasks, it notably affects the accuracy of the regression, which can significantly impact downstream tasks that require high precision, such as clustering and anomaly detection.

\begin{table}[h]
\centering
\caption{Comparison of the approximation errors.}
\small 
\label{tab:appro_err}
\begin{tabular}{c|l|ccc}
\hline
\multirow{2}{*}{\textbf{Dataset}} & \multirow{2}{*}{\textbf{Model}} & \multicolumn{3}{c}{\textbf{Approximate Error ($\times 10^{-3}$)}}\\
\cline{3-5}
& & \textit{DTW} & \textit{Hausdorff} & \textit{Fr\'e{}chet} \\
\hline
\multirow{5}{*}{Porto} & NeuTraj~\cite{yao2019computing} & 1.8206 & 1.3871 & 1.2367 \\
& Traj2simvec~\cite{zhang2020trajectory} & 5.5506 & 0.9988 & 1.0113 \\
& T3S~\cite{yang2021t3s} & 1.6830 & 0.6674 & \underline{0.6832} \\
& TMN-NM~\cite{yang2022tmn} & \underline{1.4253} & \underline{0.6402} & 0.6980 \\
& \textbf{SIMformer (Ours)} & \textbf{0.5025} & \textbf{0.3328} & \textbf{0.3773} \\
\hline
\multirow{5}{*}{Geolife} & NeuTraj~\cite{yao2019computing} & 10.6312 & 1.9034 & 1.8183 \\
& Traj2simvec~\cite{zhang2020trajectory} & 20.3792 & 1.5654 & 1.5141 \\
& T3S~\cite{yang2021t3s} & 8.7897 & 1.9318 & 1.6828 \\
& TMN-NM~\cite{yang2022tmn} & \underline{7.5104} & \underline{0.7765} & \underline{0.9545} \\
& \textbf{SIMformer (Ours)} & \textbf{1.2964} & \textbf{0.3799} & \textbf{0.6981} \\
\hline
\multirow{5}{*}{T-Drive} & NeuTraj~\cite{yao2019computing} & 5.3339 & 2.1732 & 1.6242   \\
& Traj2simvec~\cite{zhang2020trajectory} & 11.9912 &   2.1684 & 1.9450 \\
& T3S~\cite{yang2021t3s} & 5.1998 & 2.0442 & 1.3450 \\
& TMN-NM~\cite{yang2022tmn} & \underline{3.491} & \underline{1.3276} & \underline{1.1323} \\
& \textbf{SIMformer (Ours)} & \textbf{1.2041} & \textbf{0.3931} & \textbf{0.9483} \\
\hline
\multirow{5}{*}{AIS} & NeuTraj~\cite{yao2019computing} & 5.5067 & 1.3272 &  1.0083  \\
& Traj2simvec~\cite{zhang2020trajectory} & 16.7978 &  0.8863 & 0.7627 \\
& T3S~\cite{yang2021t3s} & 5.8258 & 1.3258 & 0.5853 \\
& TMN-NM~\cite{yang2022tmn} & \underline{3.9228} & \underline{0.4648} & \underline{0.4850} \\
& \textbf{SIMformer (Ours)} & \textbf{0.6847} & \textbf{0.2792} & \textbf{0.3718} \\
\hline
\end{tabular}
\end{table}

\subsection{Interpretability Study} 
We conducted an \textbf{additional interpretability study} from two perspectives to further uncover the reasons for SIMformer's outstanding performance.

\begin{figure}[!h]
  \centering
  \includegraphics[width=\linewidth]{figures/porto_distance_distribution_v2.pdf}
  \caption{Visualization of similarity distribution on Porto.}
  \label{figure:distribution_vis}
\end{figure}

\begin{figure}[!h]
  \centering
  \includegraphics[width=\linewidth]{figures/attention_score_jiang.pdf}
  \caption{Visualization of attention score on Porto.}
  \label{figure:atte_vis}
\end{figure}

\noindent \textbf{Perspective 1: Attention Heatmap.} In SIMformer, the output trajectory representation can be considered as a weighted sum of individual trajectory points' representations, determined by the model's attention scores. We randomly selected a trajectory from the Porto test set and obtained the corresponding attention scores assigned by two versions of SIMformer: one trained with tailored representation similarity function and the other with Euclidean-based one. The resulting attention scores are visualized in \autoref{figure:atte_vis} as a heatmap, where redder areas indicate higher attention scores.

As depicted in \autoref{figure:atte_vis}, for DTW, the model trained with the tailored similarity function effectively captures global key points, while the one trained with a Euclidean-based function overly emphasizes one side of the trajectory. Since DTW measures the global cumulative distance, the tailored function aligns better with this goal, resulting in a higher hit ratio (HR@50) of 0.68 compared to 0.54 for the Euclidean-based one. Similarly, for Hausdorff and Fr\'e{}chet, the model trained with the tailored similarity function focuses on critical local segments, such as the start and end parts of the trajectory. In contrast, the model trained with a Euclidean-based function lacks this focused attention. Because both Hausdorff and Fr\'e{}chet distance emphasizes the key local features of the trajectory, the attention score from tailored function better aligns with their objectives. This alignment results in significantly higher hit ratios for the tailored function (0.86 and 0.90) compared to the Euclidean-based one (0.48 and 0.68). Therefore, compared to Euclidean-based similarity functions, tailored one can better capture key trajectory information specific to each measure, leading to better performance.

\noindent \textbf{Perspective 2: Distribution Similarity.}
A good trajectory similarity learning model should be able to better capture the distribution characteristics of similarity in the original data. To this end, we visualized the ground truth similarity distribution of three distance measures on the Porto test set and the corresponding distributions learned by the models (by computing the pair-wise representation similarities). \autoref{figure:distribution_vis} shows the results. The horizontal axis represents the similarity score (ranging from 0 to 1), and the vertical axis represents the frequency of occurrences within each interval. The blue distributions indicate the ground truth, while the yellow ones indicate what the model has learned. Specifically, the upper part in yellow shows the distribution learned with Euclidean-based similarity function, and the bottom part depicts the distribution learned with tailored similarity function. The similarity distributions for all three distance measures are displayed separately. It's evident to find that the distribution learned by SIMformer (based on tailored similarity functions) is significantly better than that learned using Euclidean-based similarity functions. The tailored approach accurately captures the irregular local distribution features in the data, while the Euclidean-based approach results in a smoother distribution. This highlights the superior distribution approximation capabilities of SIMformer.

\subsection{Effectiveness in Ranking Error}
\begin{table*}[!t] 
\centering
\small
\caption{Effectiveness in ranking error ($\downarrow$) across all four datasets $\times$ three distance measures.}
\label{tab:ranking_error_all}
\resizebox{\textwidth}{!}{
\begin{tabular}{c|c|cccc|cccc|cccc}
% \toprule
\hline 
\multirow{2}{*}{\textbf{Dataset}} & \multirow{2}{*}{\textbf{Model}} & \multicolumn{4}{c|}{\textbf{Ranking Error@DTW}} & \multicolumn{4}{c|}{\textbf{Ranking Error@Hausdorff}} & \multicolumn{4}{c}{\textbf{Ranking Error@Fr\'e{}chet}} \\
 & & \textit{k=10} & \textit{k=20} & \textit{k=50} & \textit{k=100} & \textit{k=10} & \textit{k=20} & \textit{k=50} & \textit{k=100} & \textit{k=10} & \textit{k=20} & \textit{k=50} & \textit{k=100} \\
\hline 
 \multirow{8}{*}{Porto} & NeuTraj~\cite{yao2019computing} & 15.75 & 64.89 & 399.92 & 1543.90 & 16.12 & 67.24 & 423.98 & 1643.34 & 15.23 & 61.49 & 364.74 & 1357.41 \\
 & Traj2simvec~\cite{zhang2020trajectory} & 16.29 & 65.89 & 400.09 & 1528.22 & 14.89 & 62.03 & 391.55 & 1526.35 & 14.35 & 57.81 & 343.87 & 1297.75 \\
 & T3S~\cite{yang2021t3s}  & 16.26 & 66.43 & 406.03 & 1552.41 & 15.49 & 62.96 & 376.12 & 1394.67 & 14.39 & 57.40 & 338.65 & 1257.39 \\
 & TMN-NM~\cite{yang2022tmn} & 16.26 & 65.97 & 401.92 & 1532.77 & 15.03 & 60.70 & 362.67 & 1342.57 & 14.57 & 58.36 & 345.03 & 1279.75 \\
  \cline{2-14}
 & SIMformer \textit{w/ Euc.} & 16.07 & 65.18 & 398.30 & 1518.62 & 14.18 & \cellcolor{grey!20}56.84 & 343.84 & 1289.51 & 14.27 & 57.56 & 344.53 & 1284.90 \\
  & SIMformer \textit{w/ Cos.} & \textbf{14.30} & \textbf{56.58} & \textbf{326.53} & \textbf{1185.95} & \cellcolor{grey!20}14.14 & 56.98 & \cellcolor{grey!20}342.07 & \cellcolor{grey!20}1283.07 & \cellcolor{grey!20}14.11 & \cellcolor{grey!20}56.40 & \cellcolor{grey!20}336.33 & \cellcolor{grey!20}1263.00 \\ 
 & SIMformer \textit{w/ Cheby.} & \cellcolor{grey!20}15.67 & \cellcolor{grey!20}63.44 & \cellcolor{grey!20}384.22 & \cellcolor{grey!20}1457.39 & \textbf{12.70} & \textbf{49.41} & \textbf{278.79} & \textbf{984.27} & \textbf{12.15} & \textbf{47.06} & \textbf{261.61} & \textbf{902.05} \\
 \cline{2-14}
 & \emph{Improvement}  & 8.73\% & 10.81\% & 15.01\% & 18.62\% & 10.17\% & 13.08\% & 18.50\% & 23.29\% & 13.88\% & 16.57\% & 22.22\% & 28.26\% \\
\hline 
\hline
\multirow{8}{*}{Geolife} & NeuTraj~\cite{yao2019computing} & \cellcolor{grey!20}17.01 & \cellcolor{grey!20}70.54 & \cellcolor{grey!20}443.92 & 1736.94 & 16.87 & 70.40 & 437.32 & 1652.93 & 15.30 & 62.45 & 370.99 & 1325.93 \\
 & Traj2simvec~\cite{zhang2020trajectory} & 17.49 & 72.74 & 448.81 & 1749.57 & 16.20 & 67.41 & 412.12 & 1587.34 & 15.08 & 61.21 & 361.90 & 1296.53 \\
 & T3S~\cite{yang2021t3s}  & 18.03 & 74.88 & 471.60 & 1840.77 & 17.90 & 73.82 & 439.66 & 1681.85 & 15.26 & 61.81 & 364.44 & 1291.14 \\
 & TMN-NM~\cite{yang2022tmn} & 17.31 & 71.61 & 455.04 & 1783.74 & 15.93 & 65.10 & 377.88 & 1429.01 & 15.95 & 64.70 & 378.15 & 1367.96 \\ \cline{2-14}
&SIMformer \textit{w/ Euc.} & 17.05 & 70.70 & 445.11 & \cellcolor{grey!20}1733.46 & \cellcolor{grey!20}14.67 & \cellcolor{grey!20}58.53 & \cellcolor{grey!20}338.30 & \cellcolor{grey!20}1260.08 & \cellcolor{grey!20}14.93 & \cellcolor{grey!20}59.90 & \cellcolor{grey!20}352.58 & \cellcolor{grey!20}1257.41 \\
& SIMformer \textit{w/ Cos.} & \textbf{15.73} & \textbf{65.00} & \textbf{403.35} & \textbf{1562.47} & 15.32 & 62.15 & 366.29 & 1402.35 & 15.68 & 64.27 & 389.46 & 1461.40 \\ 
&SIMformer \textit{w/ Cheby.} & 17.79 & 74.55 & 469.93 & 1842.85 & \textbf{13.92} & \textbf{54.61} & \textbf{304.20} & \textbf{1090.96} & \textbf{14.61} & \textbf{58.14} & \textbf{333.66}& \textbf{1144.79} \\ \cline{2-14}
 & \emph{Improvement} & 7.52\% & 7.85\% & 9.14\% & 9.86\% & 5.15\% & 6.70\% & 10.08\% & 13.42\% & 2.19\% & 2.94\% & 5.37\% & 8.96\% \\
% \bottomrule
\hline
\hline 
\multirow{8}{*}{T-Drive} & NeuTraj~\cite{yao2019computing} & 18.37 & 76.53 & 481.31 & 1909.12 & 18.61 & 77.04 & 472.20 & 1792.75 & 17.43 & 70.46 & 425.96 & 1623.77 \\
 & Traj2simvec~\cite{zhang2020trajectory} & 18.65 & 77.50 & 483.69 & 1888.40 & 18.43 & 75.81 & 463.25 & 1763.24 & 17.51 & 71.34 & 432.07 & 1643.54 \\
 & T3S~\cite{yang2021t3s}  & 19.08 & 78.84 & 490.94 & 1921.10 & 18.09 & 72.64 & 432.92 & 1622.70 & 16.68 & 67.40 & 402.15 & 1521.50 \\
 & TMN-NM~\cite{yang2022tmn} & 18.88 & 78.05 & 488.40 & 1909.71 & 17.68 & 71.06 & 419.63 & 1557.82 & 16.71 & 67.00 & 399.67 & 1508.52 \\ \cline{2-14}
& SIMformer \textit{w/ Euc.} & 18.38 & 76.05 & 474.92 & 1858.22 & \cellcolor{grey!20}15.39 & \cellcolor{grey!20}61.48 & \cellcolor{grey!20}360.89 & \cellcolor{grey!20}1345.63 & \cellcolor{grey!20}16.25 & \cellcolor{grey!20}65.46 & \cellcolor{grey!20}389.42 & \cellcolor{grey!20}1472.99 \\
& SIMformer \textit{w/ Cos.} & \textbf{17.03} & \textbf{70.96} & \textbf{441.15} & \textbf{1700.74} & 15.59 & 63.30 & 379.57 & 1444.66 & 16.79 & 68.90 & 424.16 & 1647.81 \\ 
&SIMformer \textit{w/ Cheby.} & \cellcolor{grey!20}17.97 & \cellcolor{grey!20}73.80 & \cellcolor{grey!20}456.77 & \cellcolor{grey!20}1763.60 & \textbf{14.01} & \textbf{53.67}& \textbf{296.37} & \textbf{1038.56} & \textbf{14.91} & \textbf{58.61} & \textbf{335.91} & \textbf{1219.53} \\ \cline{2-14}
 & \emph{Improvement} & 5.26\% & 3.85\% & 3.42\% & 3.56\% & 8.97\% & 12.71\% & 17.88\% & 22.82\% & 8.22\% & 10.46\% & 13.74\% & 17.21\% \\
\hline
\hline 
 \multirow{8}{*}{AIS} & NeuTraj~\cite{yao2019computing} & 17.46 & 72.38 & 450.68 & 1738.28 & 17.77 & 73.54 & 455.90 & 1733.39 & 15.76 & 62.40 & 368.95 & 1362.32 \\
 & Traj2simvec~\cite{zhang2020trajectory} & 17.55 & 72.34 & 447.70 & 1731.01 & 15.73 & 64.97 & 396.37 & 1476.34 & 14.50 & 56.68 & 329.65 & 1197.70 \\
 & T3S~\cite{yang2021t3s}  & 18.03 & 73.99 & 451.38 & 1726.50 & 18.99 & 78.21 & 475.22 & 1759.91 & 15.07 & 58.88 & 337.28 & 1225.17 \\
 & TMN-NM~\cite{yang2022tmn} & 17.43 & 71.74 & 442.63 & 1705.53 & 16.21 & 64.64 & 375.27 & 1333.17 & 14.69 & 56.85 & \cellcolor{grey!20}326.33 & \cellcolor{grey!20}1179.07 \\ \cline{2-14}
&SIMformer \textit{w/ Euc.} & 17.31 & 71.24 & 441.47 & 1692.67 & \cellcolor{grey!20}15.42 & \cellcolor{grey!20}60.38 & \cellcolor{grey!20}341.05 & \cellcolor{grey!20}1200.95 & \cellcolor{grey!20}14.47 & \cellcolor{grey!20}56.59 & 327.77 & 1191.59 \\
& SIMformer \textit{w/ Cos.} & \textbf{16.26} & \textbf{66.06} & \textbf{399.56} & \textbf{1483.37} & 16.37 & 66.25 & 396.13 & 1453.90 & 16.14 & 64.83 & 391.41 & 1465.72 \\ 
& SIMformer \textit{w/ Cheby.} & \cellcolor{grey!20}17.10 & \cellcolor{grey!20}70.13 & \cellcolor{grey!20}426.67 & \cellcolor{grey!20}1618.87 & \textbf{14.59} & \textbf{56.73} & \textbf{315.04} & \textbf{1086.70} & \textbf{13.87} & \textbf{53.40} & \textbf{303.98} & \textbf{1062.04} \\ \cline{2-14}
 & \emph{Improvement} & 4.91\% & 5.81\% & 6.35\% & 8.37\% & 5.40\% & 6.04\% & 7.63\% & 9.51\% & 4.10\% & 5.64\% & 6.85\% & 9.93\% \\
% \bottomrule
\hline
\end{tabular}
}
\end{table*}
Due to page limitation, it is not practical to present a comprehensive table with ranking errors for all four datasets $\times$ three distance measures in the main paper body. We have attached the complete results (\autoref{tab:ranking_error_all}) here for readers' reference. These results further confirm that SIMformer's exceptional ranking performance is attributed to its utilization of both the \textit{simple pair-wise MSE loss} and the \textit{tailored representation similarity function}.
